# Supplementary material for: A magnetic Hofstadter butterfly and its topologically quantized Hall conductance
Source: arXiv:1808.00861 source file (2018-08-02)
Supplement: Supplementary file 1 [file supplementary070718_sg.pdf]

# Supplemental material
# A magnetic Hofstadter butterfly and its topologically quantized Hall conductance

Manisha Arora and Sankalpa Ghosh[1]

[1]Department of Physics, Indian Institute of Technology Delhi, New Delhi-110016, India

## I. PROOFS RELATED TO $B_p\hat{z}$ AND $\boldsymbol{A}_p$

### A. Flux due to $B_p\hat{z}$ in Eq. (4) through unit cell

$$\int_{\text{unit cell}} B_p\hat{z}\cdot d\boldsymbol{s} = \frac{(B_1-B_2)(1-\frac{\pi Rs^2}{a^2})\pi Rs^2-(B_1-B_2)\frac{\pi Rs^2}{a^2}(a^2-\pi Rs^2)}{a^2} = 0 \tag{1}$$

### B. Explicit construction of profile of the vector potential $\boldsymbol{A}_p(\boldsymbol{r})$

Consider the magnetic field profile

$$B_s\hat{z} = \Big[\frac{B_2}{N}+(B_1-B_2)\Theta(R^s-r_{m,n})\Big]\hat{\boldsymbol{z}} \tag{2}$$

depicted in Fig. 1. A superposition of such magnetic field profile through summation over all allowed values of m,n will generate the magnetic field profile $\boldsymbol{B}$ given by Eq. (1) in the main paper. To evaluate the vector potential corresponding to $\boldsymbol{B}$, we first calculate the vector potential corresponding to $B_s\hat{z}$ given in Eq. (2). Then we superpose all such vector potentials corresponding to different sets of $(m,n)$. Now, the magnetic field profile in Fig. 1 suggests that it is possible to write the vector potential purely with an azimuthal component. Accordingly, we write

$$\int \frac{\boldsymbol{B}_s.\boldsymbol{dS}}{\Phi_0} = \int \frac{\boldsymbol{A}_s.\boldsymbol{dl}}{\Phi_0} \tag{3}$$

where $\boldsymbol{A}_s$ is the vector potential only having azimuthal component. Here $\Phi_o = \frac{hc}{e}$. From the above equation we straighforwardly get

$$A_{s\theta} = \frac{c\phi(r)}{er} \tag{4}$$

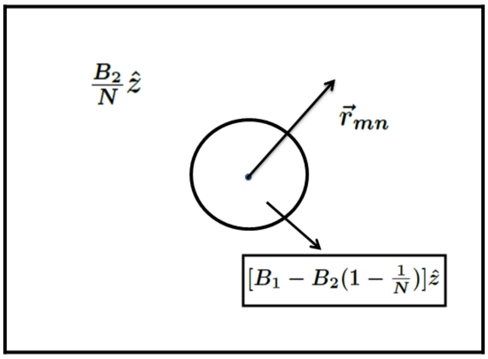


FIG. 1: Monolayer graphene under single unit magnetic field profile with inside circular region having field $[B_1-B_2(1-\frac{1}{N})]\hat{\boldsymbol{z}}$ and outside region having $\frac{B_2}{N}\hat{\boldsymbol{z}}$. Radius of the circular region is $R^s$.

where $\phi(r)$ is given as

$$\phi(r) = \begin{cases} \frac{e}{c}[\frac{B_2}{N}\frac{r^2}{2} + \frac{(B_1-B_2)r^2}{2}], & \text{if } r \leq R^s \\ \frac{e}{c}[\frac{B_2}{N}\frac{r^2}{2} + \frac{(B_1-B_2)(R^s)^2}{2}], & \text{otherwise} \end{cases} \tag{5}$$

It may be pointed out in the cases like this ( Eq. 2 ) where magnetic field profile contains a step function one adopted this technique based on Stoke's theorem to calculate the corresponding vector potential. For example see the ref. 17 in the main paper.

Hence, from Eqn. (4), we can write

$$A_{s\theta}(r) = \begin{cases} [\frac{B_2}{N}\frac{r}{2} + \frac{(B_1-B_2)r^2}{2r}], & \text{if } r \leq R^s \\ [\frac{B_2}{N}\frac{r}{2} + \frac{(B_1-B_2)(R^s)^2}{2r}], & \text{otherwise} \end{cases}$$

From this, we find that for a given $(m, n)$ the azimuthal component of the vector potential is given as

$$A_{mn} = \begin{cases} [\frac{B_2}{N}\frac{r_{mn}}{2} + \frac{(B_1-B_2)r_{mn}^2}{2r_{mn}}], & \text{if } r_{mn} \leq R^s \\ [\frac{B_2}{N}\frac{r_{mn}}{2} + \frac{(B_1-B_2)(R^s)^2}{2r_{mn}}], & \text{otherwise} \end{cases} \tag{6}$$

where $r_{mn}$ and $R^s$ are defined in the main document. Thus, the total vector potential for the field profile $\boldsymbol{B}$ can be written as

$$\boldsymbol{A}(\boldsymbol{r}) = \sum_{m,n}[(\boldsymbol{A}_{mn}.\hat{\boldsymbol{x}})\hat{\boldsymbol{x}} + (\boldsymbol{A}_{mn}.\hat{\boldsymbol{y}})\hat{\boldsymbol{y}}]$$

Since $B\hat{z} = B_u\hat{\boldsymbol{z}} + B_p\hat{\boldsymbol{z}}$, then upto a gauge choice vector potential (say $\boldsymbol{A}_{rem}(\boldsymbol{r})$) corresponding to $\boldsymbol{B}_p$ can be obtained as

$$\boldsymbol{A}_{rem}(\boldsymbol{r}) = \boldsymbol{A}(\boldsymbol{r}) - \boldsymbol{A}_u(\boldsymbol{r}) \tag{7}$$

where $\boldsymbol{A}_u = \frac{1}{2}(\boldsymbol{B}_u \times \boldsymbol{r})$ is given in the symmetric gauge. A straightforward but lengthy algebra involving various terms in the expression of $\boldsymbol{A}_{rem}(\boldsymbol{r}) = A_{remx}\hat{\boldsymbol{x}} + A_{remy}\hat{\boldsymbol{y}}$, shows that $\boldsymbol{A}_{rem}$ can be written as a superposition of a periodic term and another part $\boldsymbol{A}_{rem}^{rest}$ whose curl is zero. The second part can therefore be removed through a gauge transformation and this leaves us with expression for periodic vector potential $\boldsymbol{A}_p(\boldsymbol{r})$ corresponding to $\boldsymbol{B}_p$, shown in Eq. (4) of the main document.

More explicitly we can write

$$\begin{aligned} \boldsymbol{A}_p(\boldsymbol{r}) &= \frac{1}{2}\sum_{m,n}\Big[(B_p^{mn}\hat{\boldsymbol{z}}) \times (\boldsymbol{r} - \boldsymbol{R}_{mn})\Big] \\ &= \frac{1}{2}\sum_{m,n}\Big[(B_p^{mn}\hat{\boldsymbol{z}}) \times (r_{mn}\hat{\boldsymbol{r}}_{mn})\Big] \\ &= \frac{1}{2}\sum_{m,n}(B_p^{mn}r_{mn})\hat{\boldsymbol{\theta}}_{mn} \end{aligned} \tag{8}$$

where $B_p^{mn}$ is defined, in the main text, in Eq. (6). and one can show that $\boldsymbol{\nabla} \times (\boldsymbol{A}_{rem} - \boldsymbol{A}_p) = 0$.

### C. Periodicity of $\boldsymbol{A}_p(\boldsymbol{r})$

Rewriting $\boldsymbol{A}_p(\boldsymbol{r})$ from Eqn. (8) as

$$\boldsymbol{A}_p(\boldsymbol{r}) = \frac{1}{2}\sum_{m,n}\Big[(B_p^{mn}\hat{\boldsymbol{z}}) \times (\boldsymbol{r} - \boldsymbol{R}_{mn})\Big] \tag{9}$$

Now performing a lattice translation with vector $\boldsymbol{R} = la\hat{\boldsymbol{x}} + ka\hat{\boldsymbol{y}}$, we obtain

$$\boldsymbol{A}_p(\boldsymbol{r}+\boldsymbol{R}) = \frac{1}{2}\sum_{m'',n''}\left[(B_p^{m''n''}\hat{\boldsymbol{z}}) \times (\boldsymbol{r} - \boldsymbol{R}_{m''n''})\right] \tag{10}$$

where $m'' = (m-l)$ and $n'' = (n-k)$ and the limits are $m'' = (-Nmax - l) : (Nmax - l)$ and $n'' = (-Nmax - k) : (Nmax - k)$. Thus

$$\boldsymbol{A}_p(\boldsymbol{r}+\boldsymbol{R}) = \boldsymbol{A}_p(\boldsymbol{r}) \tag{11}$$

## II. DERIVATION OF EQ. (12) FROM EQ. (9) IN THE MAIN PAPER

### A. Discretization and implementation of the weak magnetic field condition

Consider the Taylor expansion

$$\psi(x+a) = \psi(x) + a\frac{\partial\psi(x)}{\partial x} + \frac{a^2}{2!}\frac{\partial^2\psi(x)}{\partial x^2} + .. \tag{12}$$

For a slowly varying function, therefore

$$a\frac{\partial\psi(x)}{\partial x} + \frac{a^2}{2!}\frac{\partial^2\psi(x)}{\partial x^2} \sim \psi(x+a) - \psi(x) \tag{13}$$

Define the dimensionless variable and the functions in terms of them as

$$\bar{x} = \frac{x}{l_{Bu}}, \phi(\bar{x}) = \psi(x) \tag{14}$$

where $\ell_{B_u}$ is the magnetic length corresponding to the uniform magnetic field $B_u\hat{z}$. Now

$$\begin{aligned}\frac{\partial\psi(x)}{\partial x} &= \frac{1}{l_{Bu}}\frac{\partial\phi(\bar{x})}{\partial\bar{x}} \\ \frac{\partial^2\psi(x)}{\partial x^2} &= \frac{1}{l_{Bu}^2}\frac{\partial^2\phi(\bar{x})}{\partial^2\bar{x}}\end{aligned} \tag{15}$$

Now using Eqns. (14-15) in Eqn. (13) we get

$$\frac{a}{l_{Bu}}\frac{\partial\phi(\bar{x})}{\partial\bar{x}} + \frac{1}{2!}(\frac{a}{l_{Bu}})^2\frac{\partial^2\phi(\bar{x})}{\partial^2\bar{x}} = [\phi(\overline{x+a}) - \phi(\bar{x})] \tag{16}$$

For $\frac{a}{l_{Bu}} << 1$ (for the uniform magnetic field case)[1], we can even neglect terms containing $(\frac{a}{l_{Bu}})^2$ and higher orders. Thus

$$\frac{\partial\psi(x)}{\partial x} = \frac{\psi(x+a) - \psi(x)}{a} \tag{17}$$

Rewriting the condition in terms of magnetic field it reads $|\frac{ea^2B_u}{\hbar c}| \ll 1$ which is satisfied for a weak and slowly varying field This condition can be extended for the case of

$$|\frac{ea^2B(\boldsymbol{r})}{\hbar c}| << 1 \tag{18}$$

where $B(\boldsymbol{r}) = B_u + B_p(\boldsymbol{r})$. Assuming the condition in Eq. (18) is satisfied Eqn. (9) in the main text

$$\hat{H}_G(x,y)\psi^a_{\boldsymbol{k}}(x,y) = E^2\psi^a_{\boldsymbol{k}}(x,y) \tag{19}$$

can be discretized as follows :

$$\begin{aligned}(p+\frac{e}{c}A_u)^2\psi^a_{\boldsymbol{k}}(\boldsymbol{r}) &= -\hbar^2(\frac{\psi^a_{\boldsymbol{k}}(\boldsymbol{r}+a\hat{\boldsymbol{x}}) + \psi^a_{\boldsymbol{k}}(\boldsymbol{r}-a\hat{\boldsymbol{x}}) - 2\psi^a_{\boldsymbol{k}}(\boldsymbol{r})}{a^2}) - \hbar^2(\frac{\psi^a_{\boldsymbol{k}}(\boldsymbol{r}+a\hat{\boldsymbol{y}}) + \psi^a_{\boldsymbol{k}}(\boldsymbol{r}-a\hat{\boldsymbol{y}}) - 2\psi^a_{\boldsymbol{k}}(\boldsymbol{r})}{a^2}) \\ &+ \frac{e^2}{c^2}A_u^2\psi^a_{\boldsymbol{k}}(\boldsymbol{r}) - \frac{i\hbar e}{c}A_{ux}(\frac{\psi^a_{\boldsymbol{k}}(\boldsymbol{r}+a\hat{\boldsymbol{x}}) - \psi^a_{\boldsymbol{k}}(\boldsymbol{r}-a\hat{\boldsymbol{x}})}{a}) - \frac{i\hbar e}{c}A_{uy}(\frac{\psi^a_{\boldsymbol{k}}(\boldsymbol{r}+a\hat{\boldsymbol{y}}) - \psi^a_{\boldsymbol{k}}(\boldsymbol{r}-a\hat{\boldsymbol{y}})}{a})\end{aligned}$$

and

$$(\frac{e^2}{c^2}A_p^2+\frac{2e}{c}\boldsymbol{A}_p.\boldsymbol{p})\psi^a_{\boldsymbol{k}}(\boldsymbol{r}) = \frac{e^2}{c^2}A_p^2\psi^a_{\boldsymbol{k}}(\boldsymbol{r})-\frac{i\hbar e}{c}A_{px}(\frac{\psi^a_{\boldsymbol{k}}(\boldsymbol{r}+a\hat{\boldsymbol{x}})-\psi^a_{\boldsymbol{k}}(\boldsymbol{r}-a\hat{\boldsymbol{x}})}{a})-\frac{i\hbar e}{c}A_{py}(\frac{\psi^a_{\boldsymbol{k}}(\boldsymbol{r}+a\hat{\boldsymbol{y}})-\psi^a_{\boldsymbol{k}}(\boldsymbol{r}-a\hat{\boldsymbol{y}})}{a})$$

Now using these two expressions in the eigenvalue equation (19) and multiplying both sides with $\frac{-a^2}{\hbar^2}$ we get:

$$\begin{aligned}\epsilon\psi^a_{\boldsymbol{k}}(\boldsymbol{r}) &= (1+\frac{iea}{\hbar c}(A_{ux}+A_{px}))\psi^a_{\boldsymbol{k}}(\boldsymbol{r}+a\hat{\boldsymbol{x}})+(1-\frac{iea}{\hbar c}(A_{ux}+A_{px})\psi^a_{\boldsymbol{k}}(\boldsymbol{r}-a\hat{\boldsymbol{x}})\\ &+ (1+\frac{iea}{\hbar c}(A_{uy}+A_{py}))\psi^a_{\boldsymbol{k}}(\boldsymbol{r}+a\hat{\boldsymbol{y}})+(1-\frac{iea}{\hbar c}(A_{uy}+A_{py}))\psi^a_{\boldsymbol{k}}(\boldsymbol{r}-a\hat{\boldsymbol{y}})\\ &- [\frac{e^2}{\hbar^2c^2}a^2(A_u^2+A_p^2)+\frac{2e^2a^2}{\hbar^2c^2}(A_{ux}A_{px}+A_{uy}A_{py})+\frac{ea^2}{\hbar c}(B_u+B_p)+4]\psi^a_{\boldsymbol{k}}(\boldsymbol{r})\end{aligned} \tag{20}$$

where $\epsilon=\frac{-E^2a^2}{v_F^2\hbar^2}$ is the dimensionless energy. Now, as shown in Eqn. (11) of the main text, we have

$$\psi^a_{\boldsymbol{k}}(\boldsymbol{r})=\sum_i g(\boldsymbol{R}_i)w(\boldsymbol{r}-\boldsymbol{R}_i) \tag{21}$$

where $w(\boldsymbol{r}-\boldsymbol{R}_i)=\exp(-i\frac{e\boldsymbol{A}_u\cdot\boldsymbol{R}_i}{\hbar c})w_0(\boldsymbol{r}-\boldsymbol{R}_i)$ are the phase transformed Wannier functions. Defining $\boldsymbol{R}_i-a\hat{\boldsymbol{x}}=\boldsymbol{R}_l$. From Eq. (20) we get

$$\begin{aligned}\epsilon\sum_l g(\boldsymbol{R}_l)w(\boldsymbol{r}-\boldsymbol{R}_l) &= (1+\frac{iea}{\hbar c}(A_{ux}+A_{px}))\sum_l g(\boldsymbol{R}_l+a\hat{\boldsymbol{x}})w(\boldsymbol{r}-\boldsymbol{R}_l)\\ &+ (1-\frac{iea}{\hbar c}(A_{ux}+A_{px}))\sum_l g(\boldsymbol{R}_l-a\hat{\boldsymbol{x}})w(\boldsymbol{r}-\boldsymbol{R}_l)\\ &+ (1+\frac{iea}{\hbar c}(A_{uy}+A_{py}))\sum_l g(\boldsymbol{R}_l+a\hat{\boldsymbol{y}})w(\boldsymbol{r}-\boldsymbol{R}_l)\\ &+ (1-\frac{iea}{\hbar c}(A_{uy}+A_{py}))\sum_l g(\boldsymbol{R}_l-a\hat{\boldsymbol{y}})w(\boldsymbol{r}-\boldsymbol{R}_l)\\ &- [\frac{e^2}{\hbar^2c^2}a^2(A_u^2+A_p^2)+\frac{2e^2a^2}{\hbar^2c^2}(A_{ux}A_{px}+A_{uy}A_{py})\\ &+ \frac{ea^2}{\hbar c}(B_u+B_p)+4]\sum_l g(\boldsymbol{R}_l)w(\boldsymbol{r}-\boldsymbol{R}_l)\end{aligned}$$

Now multiplying both sides of the above equation with $w^*(\boldsymbol{r}-\boldsymbol{R}_j)$ and using the orthogonality property of the phase transformed wannier functions (given in subsection II (B)) we finally get

$$\begin{aligned}\epsilon g(\boldsymbol{R}_j) &= (1+\frac{iea}{\hbar c}(A_{ux}+A_{px}))g(\boldsymbol{R}_j+a\hat{\boldsymbol{x}})+(1-\frac{iea}{\hbar c}(A_{ux}+A_{px})g(\boldsymbol{R}_j-a\hat{\boldsymbol{x}})\\ &+ (1+\frac{iea}{\hbar c}(A_{uy}+A_{py}))g(\boldsymbol{R}_j+a\hat{\boldsymbol{y}})+(1-\frac{iea}{\hbar c}(A_{uy}+A_{py}))g(\boldsymbol{R}_j-a\hat{\boldsymbol{y}})\\ &- [\frac{e^2}{\hbar^2c^2}a^2(A_u^2+A_p^2)+\frac{2e^2a^2}{\hbar^2c^2}(A_{ux}A_{px}+A_{uy}A_{py})+\frac{ea^2}{\hbar c}(B_u+B_p)+4]g(\boldsymbol{R}_j)\end{aligned} \tag{22}$$

All the terms that are quadratic in vector potential can be ignored under the condition (18) in the above equation. This finally gives us the Eq. (12) in the main text, which is the famous Hofstadter-Harper Equation.

$$\begin{aligned}\epsilon g(m,n) &= e^{\frac{iea}{\hbar c}(A_{ux}+A_{px})}g(m+1,n)+e^{-\frac{iea}{\hbar c}(A_{ux}+A_{px})}g(m-1,n)+e^{\frac{iea}{\hbar c}(A_{uy}+A_{py})}g(m,n+1)\\ &+ e^{-\frac{iea}{\hbar c}(A_{uy}+A_{py})}g(m,n-1)-(\frac{ea^2}{\hbar c}(B_u+B_p)+4)g(m,n)\end{aligned} \tag{23}$$

### B. Orthogonality of phase transformed Wannier functions

For the proof of orthogonality condition, we proceed as follows

$$\begin{aligned}
I(say) &= \int w^*(\boldsymbol{r}-\boldsymbol{R}_j)w(\boldsymbol{r}-\boldsymbol{R}_l)\boldsymbol{dr} \\
&= \int e^{\frac{ie}{\hbar c}\boldsymbol{A}_u(\boldsymbol{r}).(\boldsymbol{R}_j-\boldsymbol{R}_l)}(w^0(\boldsymbol{r}-\boldsymbol{R}_j))^* w^0(\boldsymbol{r}-\boldsymbol{R}_l)\boldsymbol{dr} \\
&= \int e^{\frac{ie}{2\hbar c}(-B_u y\hat{\boldsymbol{x}}+B_u x\hat{\boldsymbol{y}}).((m-m')a\hat{\boldsymbol{x}}+(n-n')a\hat{\boldsymbol{y}})}(w^0(\boldsymbol{r}-\boldsymbol{R}_j))^* w^0(\boldsymbol{r}-\boldsymbol{R}_l)\boldsymbol{dr} \\
&= \int e^{-\frac{ie}{2\hbar c}B_u y(m-m')a}e^{-\frac{ie}{2\hbar c}B_u x(n-n')a}(w^0(x-ma,y-na))^* w^0(x-m'a,y-n'a)\boldsymbol{dr}
\end{aligned}$$

which can further be simplified as

$$\begin{aligned}
I &= \int e^{-\frac{ie}{2\hbar c}B_u y(m-m')a}e^{-\frac{ie}{2\hbar c}B_u x(n-n')a}(w^0(x-ma))^*(w^0(y-na))^* \\
&\times\ w^0(x-m'a)w^0(y-n'a)dxdy \\
&= \int e^{-\frac{ie}{2\hbar c}B_u x(n-n')a}(w^0(x-ma))^* w^0(x-m'a)dx \\
&\times \int e^{-\frac{ie}{2\hbar c}B_u y(m-m')a}(w^0(y-na))^* w^0(y-n'a)dy
\end{aligned}$$

Now, for $x$ integration, $y$-coordinate does not change, hence $n-n'=0$. Similarly for $y$ integration $m-m'=0$, which leads to

$$I = \int (w^0(x-ma))^* w^0(x-m'a)dx \int (w^0(y-na))^* w^0(y-n'a)dy$$

Now we are left with Wannier functions in absence of any magnetic field, which are orthonormal. Hence we write

$$\begin{aligned}
I &= \int (w^0(x-ma))^* w^0(x-m'a)dx \int (w^0(y-na))^* w^0(y-n'a)dy \\
&= \delta_{mm'}\delta_{nn'}
\end{aligned} \tag{24}$$

## III. QUANTIZATION OF HALL CONDUCTIVITY IN TERMS OF TOPOLOGICAL INVARIANT

The following discussion is mostly available in ref.[2]. We provide an abridged version of the same. In the main text, using Eqn. (15) in Eqn. (7) gives

$$\hat{H}(k_x,k_y)u'_{k_x,k_y} = Eu'_{k_x,k_y} \tag{25}$$

where

$$\hat{H}(k_x,k_y) = \begin{bmatrix} 0 & H_{12} \\ H_{21} & 0 \end{bmatrix}$$

with

$$H_{12} = ((-i\hbar\frac{\partial}{\partial x}+\hbar k_x+\frac{eA_x}{c}) - i(-i\hbar\frac{\partial}{\partial y}+\hbar k_y+\frac{eA_y}{c}))$$

and

$$H_{21} = ((-i\hbar\frac{\partial}{\partial x}+\hbar k_x+\frac{eA_x}{c}) + i(-i\hbar\frac{\partial}{\partial y}+\hbar k_y+\frac{eA_y}{c}))$$

Here $A_x$ and $A_y$ depict x and y components of total vector potential $\boldsymbol{A}(\boldsymbol{r})$ given in the main paper. We write Hall conductance for a completely filled band (Here we perform the calculation for a single band hence band index does not appear) as

$$\begin{aligned}\sigma_{xy} &= \frac{e^2}{h}\frac{1}{2\pi i}\int d^2k \int d^2r \Big(\frac{\partial u'^*_{k_x,k_y}}{\partial k_y}.\frac{\partial u'_{k_x,k_y}}{\partial k_x} \\ &- \frac{\partial u'^*_{k_x,k_y}}{\partial k_x}\frac{\partial u'_{k_x,k_y}}{\partial k_y}\Big)\end{aligned} \tag{26}$$

where the integrations are taken over the unit cells in r and k space. The above equation is same as the Eq. (16) in the main paper, but written explicitly in terms of the components. In the Eq. (16) of the main paper the Hall conductivity is written as a curl of a function that is function of Bloch vectors and the integration is over the magnetic Brillouin zone which has the topology of a Torus. This, Eq. (16) of the main text, can be written equivalently (using Stoke's law) as

$$\sigma_{xy} = \frac{e^2}{h}\frac{1}{2\pi i}\int_{\partial MBZ} \boldsymbol{dk}.\hat{\boldsymbol{A}}(k_x, k_y) \tag{27}$$

where the integration is over the boundary of the MBZ. Since the Torus has no boundary, this means if $\hat{\boldsymbol{A}}(k_x, k_y)$ is uniquely defined on the entire torus, it yields $\sigma_{xy} = 0$. Thus a finite Hall conductivity implies that the the function $\hat{\boldsymbol{A}}(k_x, k_y)$ cannot be uniquely defined on this space. Now, for understanding the non trivial topology of $\hat{\boldsymbol{A}}(k_x, k_y)$, we consider the gauge transformation

$$\begin{bmatrix} u^{aa}_{k_x,k_y} \\ u^{bb}_{k_x,k_y}\end{bmatrix} = e^{if(k_x,k_y)}\begin{bmatrix} u^{a}_{k_x,k_y} \\ u^{b}_{k_x,k_y}\end{bmatrix} \tag{28}$$

where $f(k_x, k_y)$ is some arbitrary smooth function of only $k_x$ and $k_y$. We can see that this transformation changes the phase of the wave-function but leaves the physical quantity like Hall conductivity invariant. Now, as $u'_{k_x,k_y}$ vanishes for some $(k_x, k_y)$ in the torus (Magnetic Bloch functions have zeros), the transformation given by Eq.(28) cannot be defined over the entire MBZ uniquely. Let us consider the simplest case of a single zero of $u'_{k_x,k_y}$ in the MBZ. We divide the MBZ into two regions using a circular boundary such that inside region (say region I) has a zero of the function $u'_{k_x,k_y}(x, y)$, say $\boldsymbol{k} = \boldsymbol{k}_0$, and outside region (say region II) does not have a zero. Thus for region I, we define some other function $u''_{k_x,k_y}$ which is non zero everywhere in this region. Hence for region I, say $H_I$, we can write

$$\begin{bmatrix} u^{a1}_{k_x,k_y} \\ u^{b1}_{k_x,k_y}\end{bmatrix} = e^{ig(k_x,k_y)}\begin{bmatrix} u^{a}_{k_x,k_y} \\ u^{b}_{k_x,k_y}\end{bmatrix}$$

and for region II, say $H_{II}$, we can have

$$\begin{bmatrix} u^{a2}_{k_x,k_y} \\ u^{b2}_{k_x,k_y}\end{bmatrix} = e^{ih(k_x,k_y)}\begin{bmatrix} u^{a}_{k_x,k_y} \\ u^{b}_{k_x,k_y}\end{bmatrix}$$

Eq. (16 ) in the main paper now becomes

$$\begin{aligned}\sigma_{xy} &= \frac{e^2}{h}\frac{1}{2\pi i}\Big[\int_{H_1} d^2k[\boldsymbol{\nabla}\times\hat{\boldsymbol{A}}^1(k_x, k_y)]_3 \\ &+ \int_{H_2} d^2k[\boldsymbol{\nabla}\times\hat{\boldsymbol{A}}^2(k_x, k_y)]_3\Big]\end{aligned} \tag{29}$$

where the vectors $\hat{\boldsymbol{A}}^1(k_x, k_y)$ and $\hat{\boldsymbol{A}}^2(k_x, k_y)$ are defined for regions I and II respectively and can be explicitly written as

$$\begin{aligned}\hat{\boldsymbol{A}}^1(k_x, k_y) &= \int d^2r[\hat{\boldsymbol{k_x}}(i\frac{\partial g}{\partial k_x}u^{a*}_{k_x,k_y}u^{a}_{k_x,k_y} + i\frac{\partial g}{\partial k_x}u^{b*}_{k_x,k_y}u^{b}_{k_x,k_y} + u^{a*}_{k_x,k_y}\frac{\partial}{\partial k_x}u^{a}_{k_x,k_y} + u^{b*}_{k_x,k_y}\frac{\partial}{\partial k_x}u^{b}_{k_x,k_y}) \\ &+ \hat{\boldsymbol{k_y}}(i\frac{\partial g}{\partial k_y}u^{a*}_{k_x,k_y}u^{a}_{k_x,k_y} + i\frac{\partial g}{\partial k_y}u^{b*}_{k_x,k_y}u^{b}_{k_x,k_y} + u^{a*}_{k_x,k_y}\frac{\partial}{\partial k_y}u^{a}_{k_x,k_y} + u^{b*}_{k_x,k_y}\frac{\partial}{\partial k_y}u^{b}_{k_x,k_y})]\end{aligned} \tag{30}$$

and

$$\hat{\boldsymbol{A}}^2(k_x,k_y) = \int d^2r[\hat{\boldsymbol{k_x}}(i\frac{\partial h}{\partial k_x}u^{a*}_{k_x,k_y}u^a_{k_x,k_y} + i\frac{\partial h}{\partial k_x}u^{b*}_{k_x,k_y}u^b_{k_x,k_y} + u^{a*}_{k_x,k_y}\frac{\partial}{\partial k_x}u^a_{k_x,k_y} + u^{b*}_{k_x,k_y}\frac{\partial}{\partial k_x}u^b_{k_x,k_y})$$
$$+ \hat{\boldsymbol{k_y}}(i\frac{\partial h}{\partial k_y}u^{a*}_{k_x,k_y}u^a_{k_x,k_y} + i\frac{\partial h}{\partial k_y}u^{b*}_{k_x,k_y}u^b_{k_x,k_y} + u^{a*}_{k_x,k_y}\frac{\partial}{\partial k_y}u^a_{k_x,k_y} + u^{b*}_{k_x,k_y}\frac{\partial}{\partial k_y}u^b_{k_x,k_y})] \tag{31}$$

Here we have used $u^a_{k_x,k_y}$ and $u^b_{k_x,k_y}$ to be the normalized eigenfunctions. From (30) and (31), we get

$$\hat{\boldsymbol{A}}^1(k_x,k_y) - \hat{\boldsymbol{A}}^2(k_x,k_y) = 2i\boldsymbol{\nabla_k}t(\boldsymbol{k}) \tag{32}$$

where $t(\boldsymbol{k}) = g(\boldsymbol{k}) - h(\boldsymbol{k})$. We now write, using Stokes theorem and the fact that the two regions have opposite directions for circulation, the Eqn. (29) as

$$\sigma_{xy} = \frac{e^2}{h}\frac{1}{2\pi i}\int_C \boldsymbol{dk}.(\hat{\boldsymbol{A}}^1(k_x,k_y) - \hat{\boldsymbol{A}}^2(k_x,k_y)) \tag{33}$$

which on using Eqn. (32) leads to

$$\sigma_{xy} = \frac{2e^2}{h}\frac{1}{2\pi}\int_C \boldsymbol{dk}.\boldsymbol{\nabla_k}t(\boldsymbol{k}) \tag{34}$$

where $C$ denotes closed boundary between the two regions. At each point on the closed loop C, the wavefunction has to be single valued therefore after traversing the complete loop C the two wavefunctions still should have the same phase relationship. This is possible if only

$$\begin{bmatrix} u^{a2}_{k_x,k_y} \\ u^{b2}_{k_x,k_y} \end{bmatrix} = e^{i(t(k_x,k_y)+2\pi\sigma_H)}.\begin{bmatrix} u^{a1}_{k_x,k_y} \\ u^{b1}_{k_x,k_y} \end{bmatrix} \tag{35}$$

where $\sigma_H$ is an integer This expression finally comes out to be

$$\sigma_{xy} = \frac{2e^2}{h}\sigma_H \tag{36}$$

where $\sigma_H$ is an integer. Here the factor 2 comes from the sublattice degrees of freedom

## IV. DIOPHANTINE EQUATION

The integral in the Eq. (27) is actually the Berry phase / gauge invariant geometric phase accumulated by the wavefunction in the reciprocal space[3]

$$\gamma = \oint_C \boldsymbol{dk}.\hat{\boldsymbol{A}}(k_x,k_y) \tag{37}$$

Written explicitly over the contour defined in Fig. 2

$$
\begin{aligned}
\gamma &= \int_{C_1} dk_x \int [{u^a}^*_{k_x,k_y} \frac{\partial {u^a}_{k_x,k_y}}{\partial k_x} \\
&+ {u^b}^*_{k_x,k_y} \frac{\partial {u^b}_{k_x,k_y}}{\partial k_x}] dxdy \\
&+ \int_{C_2} dk_y \int [{u^a}^*_{k_x,k_y} \frac{\partial {u^a}_{k_x,k_y}}{\partial k_y} \\
&+ {u^b}^*_{k_x,k_y} \frac{\partial {u^b}_{k_x,k_y}}{\partial k_y}] dxdy \\
&+ \int_{C_3} dk_x \int [{u^a}^*_{k_x,k_y} \frac{\partial {u^a}_{k_x,k_y}}{\partial k_x} \\
&+ {u^b}^*_{k_x,k_y} \frac{\partial {u^b}_{k_x,k_y}}{\partial k_x}] dxdy \\
&+ \int_{C_4} dk_y \int [{u^a}^*_{k_x,k_y} \frac{\partial {u^a}_{k_x,k_y}}{\partial k_y} \\
&+ {u^b}^*_{k_x,k_y} \frac{\partial {u^b}_{k_x,k_y}}{\partial k_y}] dxdy \qquad (38)
\end{aligned}
$$

where we take one of the MBZs out of the following

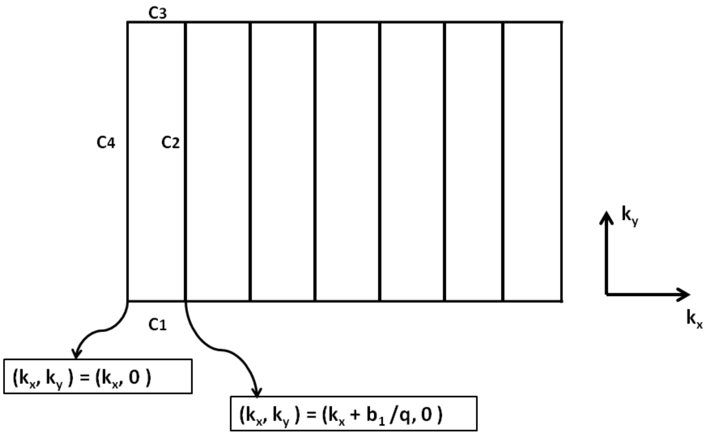


FIG. 2: Magnetic Brillouin zone

Even though the integral defined in the Eq. (27) is a gauge invariant quantity, Berry connection $\boldsymbol{A}$ is not unique. To fix it the following construction for parallel transportation[5] is done

$$\int u^*_{k_x,k_y} \frac{\partial u_{k_x},k_y}{\partial k_y} dxdy = 0 \qquad (39)$$

and

$$\int u^*_{k_x,0} \frac{\partial u_{k_x,0}}{\partial k_x} dxdy = 0 \qquad (40)$$

Eq. (39) renders the second and fourth term in the expression (38) to zero and Eq. (40) makes the contribution from the first term zero[6]. This contribution makes the phases of the wavefunction satisfy

$$
\begin{aligned}
u_{k_x+\frac{b_1}{q},k_y} &= u_{k_x,k_y} \qquad (41) \\
u_{k_x,k_y+b_2} &= e^{i\delta(k_x)} u_{k_x,k_y} \qquad (42)
\end{aligned}
$$

where $\delta(k_x)$ is the $k_x$ dependent phase factor. The total phase change around MBZ therefore need to satisfy

$$i\delta(k_x+\frac{b_1}{q})-i\delta(k_x)=2\pi i\times integer \tag{43}$$

Considering the contribution from the both sub-lattices we can therefore write

$$\int_{\partial MBZ}\boldsymbol{dk}.\hat{\boldsymbol{A}}(k_x,k_y)=4\pi i\times integer \tag{44}$$

However from Kubo formula it was also shown that

$$\int_{\partial MBZ}\boldsymbol{dk}.\hat{\boldsymbol{A}}(k_x,k_y)=4\pi i\sigma_H \tag{45}$$

Thus we can identify this integer as $\sigma_H$ which enables us to write Eqn. (43) as

$$\delta(k_x+\frac{b_1}{q})=\delta(k_x)+2\pi\sigma_H \tag{46}$$

The boundary conditions (41) and (42) along with Eq. 46) can now be used to set the following conditions on Magnetic Bloch functions $\psi_{k_x,k_y}$(or $\psi_{\boldsymbol{k}}$)[7,8] given in in the main paper, namely

$$\psi_{k_x+\frac{b_1}{q},k_y} = \psi_{k_x,k_y} \tag{47}$$

$$\psi_{k_x,k_y+b_2} = e^{i\sigma_H k_x qa}\psi_{k_x,k_y} \tag{48}$$

But the magnetic Bloch functions, being the eigenstates of the magnetic translational operator ( defined in Eq. (8) of the main paper) also obey the group properties of magnetic translational group ( given in Eqs. (13) of the main paper). Using them we get

$$M(qa\hat{\boldsymbol{x}})\psi_{\boldsymbol{k}} = e^{i\boldsymbol{k}.qa\hat{\boldsymbol{x}}}\psi_{\boldsymbol{k}} \tag{49}$$

$$M(a\hat{\boldsymbol{y}})\psi_{\boldsymbol{k}} = e^{i\boldsymbol{k}.a\hat{\boldsymbol{y}}}\psi_{\boldsymbol{k}} \tag{50}$$

and,

$$\begin{aligned} M_{\boldsymbol{R}_1}M_{\boldsymbol{R}_2}\psi_{\boldsymbol{k}} &= M_{\boldsymbol{R}_2}M_{\boldsymbol{R}_1}e^{2\pi i\frac{p}{q}}\psi_{\boldsymbol{k}} \\ &= M_{\boldsymbol{R}_2}e^{2\pi i\frac{p}{q}}M_{\boldsymbol{R}_1}\psi_{\boldsymbol{k}} \\ &= M_{\boldsymbol{R}_2}e^{2\pi i\frac{p}{q}}e^{i\boldsymbol{k}.a\hat{\boldsymbol{y}}}\psi_{\boldsymbol{k}} \\ &= e^{i(\boldsymbol{k}+\frac{p}{q}\boldsymbol{b}_2).a\hat{\boldsymbol{y}}}M_{\boldsymbol{R}_2}\psi_{\boldsymbol{k}} \end{aligned} \tag{51}$$

where $\boldsymbol{R}_1=a\hat{\boldsymbol{y}}$ and Eq. (50) is being used. Also for, $\boldsymbol{R}_2=a\hat{\boldsymbol{x}}$, we can write Eqn. (51) as

$$M_{a\hat{\boldsymbol{y}}}M_{a\hat{\boldsymbol{x}}}\psi_{\boldsymbol{k}}=e^{i(\boldsymbol{k}+\frac{p}{q}\boldsymbol{b}_2).a\hat{\boldsymbol{y}}}M_{a\hat{\boldsymbol{x}}}\psi_{\boldsymbol{k}} \tag{52}$$

where $M(a\hat{\boldsymbol{x}})\psi_{\boldsymbol{k}}$ depicts eigenfunction of $M(a\hat{\boldsymbol{y}})$ with eigenvalue $e^{i(\boldsymbol{k}+\frac{p}{q}\boldsymbol{b}_2).a\hat{\boldsymbol{y}}}$. Similarly $M(2a\hat{\boldsymbol{x}})\psi_{\boldsymbol{k}}$, $M(3a\hat{\boldsymbol{x}})\psi_{\boldsymbol{k}}$, $M(4a\hat{\boldsymbol{x}})\psi_{\boldsymbol{k}}$.... depict eigenfunctions of $M(a\hat{\boldsymbol{y}})$ with eigenvalues $e^{i(\boldsymbol{k}+\frac{2p}{q}\boldsymbol{b}_2).a\hat{\boldsymbol{y}}}$, $e^{i(\boldsymbol{k}+\frac{3p}{q}\boldsymbol{b}_2).a\hat{\boldsymbol{y}}}$, $e^{i(\boldsymbol{k}+\frac{4p}{q}\boldsymbol{b}_2).a\hat{\boldsymbol{y}}}$... respectively. These functions, being degenerate with $\psi_{\boldsymbol{k}}$, have same energy eigenvalues for the Hamiltonian in Eq. (7) in the main draft. Hence corresponding to each energy eigenvalue, we have q degenerate states depiciting $q$ fold degenracy of the system. Therefore we can write[7]

$$M(a\hat{\boldsymbol{x}})\psi_{\boldsymbol{k}}=e^{i\mu\boldsymbol{k}.qa\hat{\boldsymbol{x}}}\psi_{\boldsymbol{k}+\frac{p}{q}\boldsymbol{b}_2} \tag{53}$$

Here $\mu$ is an integer ( for significance of $\mu$ see[9]). Now applying $M(a\hat{\boldsymbol{x}})$ $q$ times to the above equation, we get

$$M(qa\hat{\boldsymbol{x}})\psi_{k_x,k_y}=e^{i\mu q\boldsymbol{k}.qa\hat{\boldsymbol{x}}}\psi_{k_x,k_y+pb_2} \tag{54}$$

which on using Eqs. (48) and (49) becomes

$$e^{i\boldsymbol{k}.qa\hat{\boldsymbol{x}}}\psi_{k_x,k_y}=e^{i\mu q\boldsymbol{k}.qa\hat{\boldsymbol{x}}}e^{ip\sigma_H\boldsymbol{k}.qa\hat{\boldsymbol{x}}}\psi_{k_x,k_y} \tag{55}$$

This gives

$$\mu q + \sigma_H p = 1 \tag{56}$$

which is the Diophantine equation to calculate Quantum Hall integers[10] for bands in the Energy spectrum.


[1] M. Governale and C. Ungarelli, Phys. Rev. B **58**, 7816 (1998).
[2] Mahito Kohmoto, Annals of Physics **160**, 343-354 (1984).
[3] D. J. Thouless, M. Kohmoto, M. P. Nightingale, and M. den Nijs, Phys. Rev. Lett. **49**, 405 (1982).
[4] Berry, M. V., Proc. R. Soc. London **392**, 45 (1984).
[5] D. J. Thouless, J. Phys. C: Solid State Phys. **17**, L325-L327 (1984).
[6] D. Xiao, M.-Che Chang and Qian Niu, Reviews of Mod. Phys. **82**, 1959-2006 (2010).
[7] I. Dana, Y. Avron and J. Zak, J. Phys. C: Solid State Phys. **18**, L679-L683 (1985).
[8] M. Wilkinson, J. Phys.: Cond. Mat. **10**, 7407-7427 (1998).
[9] H. Aoki and Y. Hatsugai, Phys. Rev. B **90**, 045206 (2014).
[10] Butterfly in the Quantum world, The story of most fascinating Quantum fractal, Indubala I. Satija (Morgan and Claypool Publishers, 2016), p. 10-3.
